# Supplementary material for: SOEDiff: Efficient Distillation for Small Object Editing
Source: arXiv:2405.09114 source file (2024-12-31)
Supplement: Supplementary file 1 [file appendix.tex]

\appendix

\begin{teaserfigure}
\centering
  \includegraphics[width=0.95\linewidth]{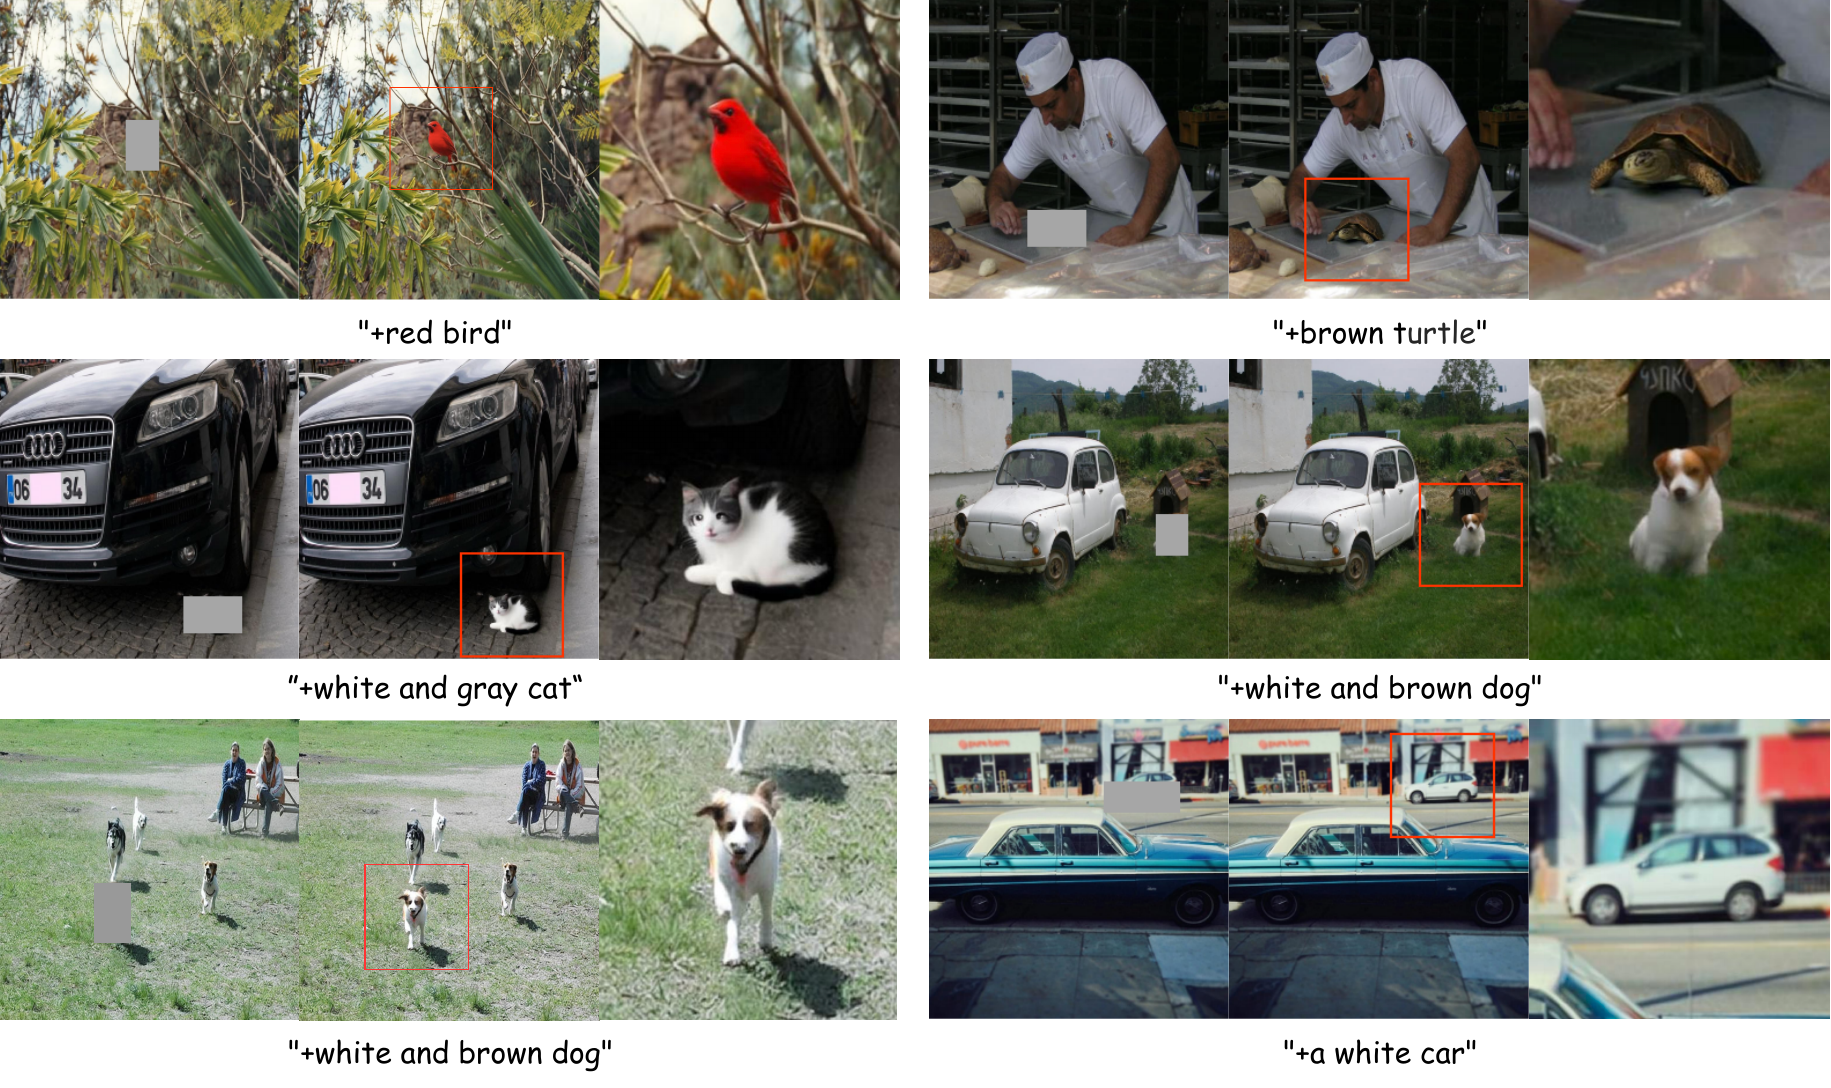}
  % \vspace{-0.5em}
  \caption{More small objects generated by our SOEDiff. The first column displays the input images and corresponding masks, the second column shows the generated images, and the third column features close-up views to highlight more detailed parts of the objects.} 
  \label{fig:teaser}
\end{teaserfigure}

\section{More Comparison Results}
We compare our method with related works (\ie, SD-I, Inpaint-Anything, HD-painter, SDXL-I)~\cite{manukyan2023hd, yu2023inpaint, avrahami2022blended, rombach2022high}, the qualitative results are shown in Fig.~\ref{fig:morecompare}. It can be observed that our method also achieves better result, mainly because this approach has inherent disadvantages, such as the loss of the overall image context information. This can sometimes lead to less effective results.

\begin{figure}[h]
\centering
  \includegraphics[width=0.95\linewidth]{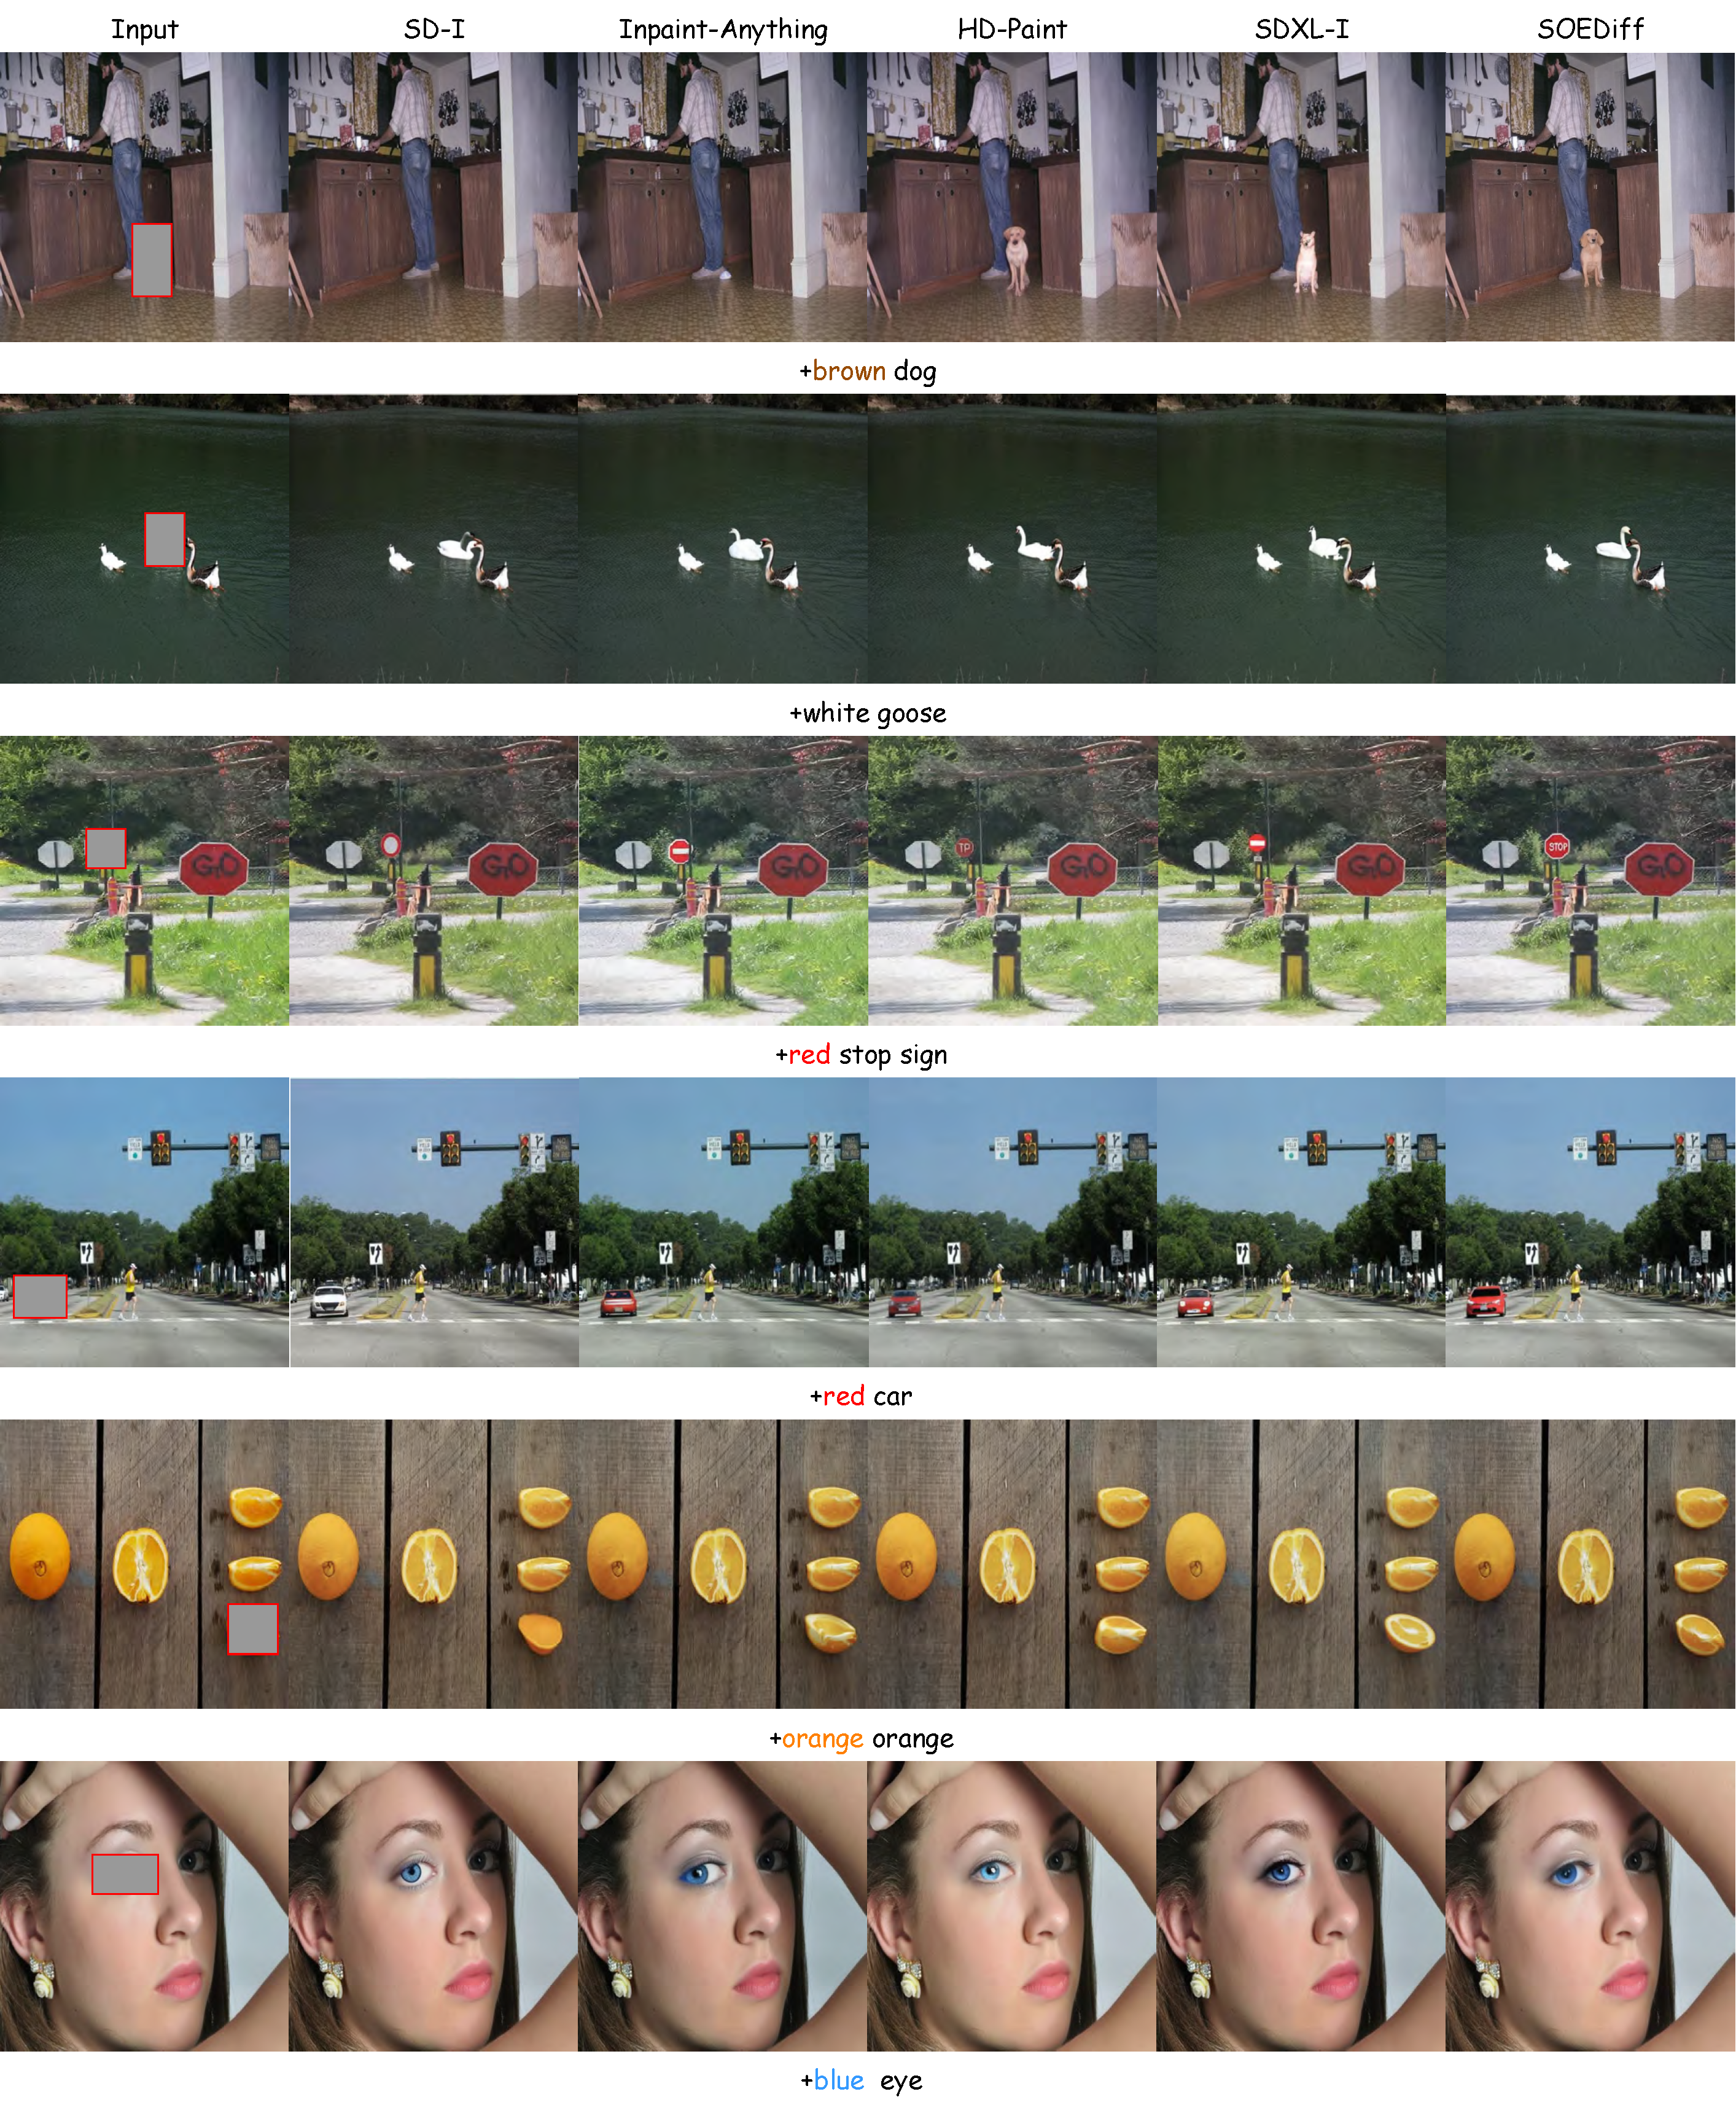}
  % \vspace{-0.5em}
  \caption{Comparing results between our methods and other models. The first column represents the input original images and corresponding masks, while the second to sixth columns show the results generated by SD-I, Inpaint-Anything, HD-painter, SDXL-I, and SOEDiff, respectively.} 
  \label{fig:morecompare}
\end{figure}

%%
%% End of file `sample-authordraft.tex'.
